# Supplementary material for: SoK: Certified Robustness for Deep Neural Networks
Source: arXiv:2009.04131 source file (2023-04-12)
Supplement: Supplementary file 1 [file appendix_old.tex]

\onecolumn
\appendix

\section{Proof of \texorpdfstring{\lowercase{\Cref{thm:bar}}}{Thm 1}}
    \label{sec:adx-omit-proof-barrier-rand-smooth}

    \begin{proof}
        % \hfill \\
        We define $g(x)_{y_0} := \bbE_{\delta\sim\mu} \left[F(x+\delta) = y_0\right]$.
        From the condition,
        $$
        \begin{aligned}
            % &  \\ 
            g(x)_{y_0} & = \int \1\left[f(x + \delta) = y_0\right]\mu(\delta) \dif \delta \\
            % g(x)_{y_0} & = \int \1\left[f(x') = y_0\right] \mu(x-x') \dif x' \\
            %  \int_{\|x'-x_0\|_p \le r} \mu(x-x') \dif x' \\
            & = \int_{\|z-(x_0-x)\|_p \le r} \mu(z) \dif z,
        \end{aligned}
        $$
        where $\mu(z)$ is the PDF of distribution $\mu$ at point $z$.
        % 
        Suppose the proposition is false, we have $g(x_0 + re_1)_{y_0} > 0.5$ and $g(x_0 - re_1)_{y_0} > 0.5$, where $e_1 = (1,0,\dots,0)^\T$ for $p < \infty$ or $e_1 = (1,1,\dots,1)^\T$ for $p = \infty$.
        Thus,
        $$
            \int_{\|z - re_1\|_p\le r} \mu(z) \dif z + \int_{\|z + re_1\|_p\le r} \mu(z) \dif z > 1.
        $$
        % It implies that
        % $
        %     \int_{\{z:\,\|z - re_1\|_p \le r\}} \mu(z)\dif z
        %     + \int_{\{z:\,\|z + re_1\|_p \le r\}} \mu(z)\dif z
        %     > 1.
        % $
        Note that $\{z:\,\|z - re_1\|_p \le r\}\cap\{z:\,\|z + re_1\|_p \le r\} = \{0\}$ has zero mass, it means that $\mu$ has probability mass $>1$ in region $\{z:\,\|z - re_1\|_p \le r\}\cup\{z:\,\|z + re_1\|_p \le r\}$, which contradicts the  definition of probability measure. 
    \end{proof}

\section{Full Taxonomy Table}
    
    \label{sec:adx-full-taxonomy-table}
    
    The full taxonomy table is shown in \Cref{tab:approach-taxonogy}.

    \begin{table*}[!t]
        \scriptsize
        \centering
        \caption{Taxonomy of neural network robustness verification and robust training approaches against $\cL_p$ adversaries.}
        
        \resizebox{0.98\textwidth}{!}{
        \begin{tabular}{c|c|c|c|c|c|c|c|c|c|c|c}
            \toprule
            \multirow{2}{*}{Approach} & \multirow{2}{*}{Main Methodologies} & \multicolumn{7}{c|}{Verification} & Robust & \multirow{2}{*}{Scalability} & \multirow{2}{*}{Base Method} \\
            \cline{3-9}
            & & Complete & Prob. & $\cL_\infty$ & $\cL_2$ & $\cL_1$ & $\cL_0$ & Other & Training & \\
            \hline \hline
            \t{Planet}~\cite{ehlers2017formal} & Branch, LP & \checkmark & & & & & & 1 & & Synthetic  \\
             \rowcolor{tabgray}
            \t{BaB}~\cite{bunel2018unified} & MILP, LP, Branch & \checkmark & & &&  & & 2 & & Synthetic & \\
            \t{BaBSR}~\cite{bunel2019branch} & LP, Branch & \checkmark & & & & & & 2 & & Synthetic & \\
             \rowcolor{tabgray}
            \t{Reluplex}~\cite{katz2017reluplex} & Branch, LP & \checkmark & & \checkmark & & & & & & MNIST &  \\
            \t{Reluval}~\cite{wang2018formal} & LP, IBP, Branch & \checkmark & & \checkmark & & & & & & MNIST & \\
             \rowcolor{tabgray}
            \t{Neurify}~\cite{wang2018efficient} & LP, Branch & \checkmark & & \checkmark & & & & & & MNIST & \\
            \t{DLV}~\cite{10.1007/978-3-319-63387-9_1} & Search & \checkmark & & & & & & 2 & & ImageNet &  \\
            
            \midrule
             \rowcolor{tabgray}
            \t{Sherlock}~\cite{dutta2017output} & MILP & \checkmark & & \checkmark & & & & & & MNIST & \\
            \t{ChengMIP}~\cite{cheng2017maximum} & MILP & \checkmark & & \checkmark & & \checkmark & & & & MNIST & \\
             \rowcolor{tabgray}
            \t{Reachability}~\cite{lomuscio2017approach} & MILP & \checkmark & & \checkmark & & & & & & MNIST & \\
            \t{Bounded MILP}~\cite{tjeng2018evaluating} & MILP & \checkmark & & \checkmark & & & & & & CIFAR-10 & \\
             \rowcolor{tabgray}
            \t{Stability}~\cite{xiao2018training} & MILP & & & & & & & & Only & CIFAR-10 & \\
            \t{AI$^2$} \cite{gehr2018ai2} & LP, Branch & \checkmark & & \checkmark & & & & & & CIFAR-10 & \\
             \rowcolor{tabgray}
            \t{GeoCert} \cite{jordan2019provable} & Lipschitz, LP & \checkmark & & \checkmark & \checkmark & \checkmark & & & & MNIST &  \\
            \midrule
            % \cite{bastani2016measuring} & LP, relax & & \checkmark & & & & & & CIFAR-10 & \\
            \t{Charon} \cite{anderson2019optimization} & LP, relax, learned & & & \checkmark & & & & & & MNIST &  \\
             \rowcolor{tabgray}
            \t{DiffAI} \cite{mirman2018differentiable} & LP, relax & & & \checkmark & & & & & \checkmark & CIFAR-10 & \\
            \t{DeepZ} \cite{singh2018fast}  & LP, relax & & & \checkmark & & & & & & CIFAR-10 & Improve from \cite{mirman2018differentiable} \\
             \rowcolor{tabgray}
            \t{DeepPoly} \cite{singh2019abstract} & LP, relax & & & \checkmark &  & & & & & CIFAR-10 &  Extend from \cite{singh2018fast} \\
            \t{RefineZono} \cite{singh2018robustness} & LP, MILP, relax & & & \checkmark & & & & & & CIFAR-10 &  Extend from \cite{singh2018fast,singh2019abstract} \\
             \rowcolor{tabgray}
            \t{k-ReLU} \cite{singh2019beyond} & LP, relax & & & \checkmark & & & & & & CIFAR-10 &  Extend from \cite{singh2018robustness} \\
            \t{Fast-Lin} \cite{weng2018towards} & LP, relax & & & \checkmark & \checkmark & \checkmark & & & & CIFAR-10 & \\
             \rowcolor{tabgray}
            \t{CROWN} \cite{zhang2018efficient} & LP, relax & & & \checkmark & \checkmark & \checkmark & & & & CIFAR-10 & Extend from \cite{weng2018towards} \\
            \t{CNN-Cert} \cite{boopathy2019cnn} & LP, relax & & & \checkmark & \checkmark & \checkmark & & & & CIFAR-10 & Extend from \cite{zhang2018efficient} \\
            % NonlinearSpec~\cite{qin2018verification} & LP, relax & & \checkmark & & & & & & CIFAR-10 & \\
             \rowcolor{tabgray}
            \t{LP-Full} \cite{weng2018towards,salman2019convex} & LP & & & \checkmark & \checkmark & & & & & MNIST & \\
            \t{C2V} \cite{tjandraatmadja2020convex} & LP, relax & & & \checkmark & & & & & & CIFAR-10 & \\
             \rowcolor{tabgray}
            \t{CROWN-IBP} \cite{zhang2020towards} & LP, IBP, relax & & & \checkmark & & & & & \checkmark & CIFAR-10 & Combine \cite{zhang2018efficient} and \cite{gowal2019scalable} \\
            \t{COLT} \cite{Balunovic2020Adversarial} & LP, relax & & & & & & & & Only & CIFAR-10 & \\
             \rowcolor{tabgray}
            \t{MMR} \cite{pmlr-v89-croce19a} & LP, relax & & & & & & & & Only & CIFAR-10 & \\
            \t{MMR-Universal} \cite{Croce2020Provable} & LP, relax & & & & & & & & Only & CIFAR-10 & \\
            \midrule
             \rowcolor{tabgray}
            \t{IBP} \cite{gowal2019scalable} & IBP & & & \checkmark & & & & & \checkmark & CIFAR-10 & \\
            \midrule
            \t{WK}~\cite{wong2018provable} & LP, dual, relax & & & \checkmark & & & & & \checkmark & MNIST & \\
             \rowcolor{tabgray}
            \t{WK+}~\cite{wong2018scaling} & LP, dual, relax & & & & & & & & Only & CIFAR-10 & \\
            \t{D-LP}~\cite{dvijotham2018dual} & LP, dual, relax & & & \checkmark & & & & & & CIFAR-10 & \\
             \rowcolor{tabgray}
            \t{PVT}~\cite{dvijotham2018training} & IBP, dual, relax, learned & & & \checkmark & & & & &
            \checkmark & CIFAR-10 & \\
            \t{Robustra} \cite{li2019robustra} & LP, dual, relax & & & & & & & & Only & CIFAR-10 & \\
             \rowcolor{tabgray}
            \t{Mixtrain} \cite{wang2018mixtrain} & LP, dual, relax & & & & & & & & Only & CIFAR-10 & \\
            \midrule
            \t{Op-norm} \cite{szegedy2013intriguing} & Lipschitz & & &  & \checkmark & & & & & CIFAR-10 & \\
             \rowcolor{tabgray}
            \t{CL} \cite{hein2017formal} & Lipschitz & & & \checkmark & \checkmark & \checkmark & & & \checkmark & CIFAR-10 & \\
            \t{Fast-Lip} \cite{weng2018towards} & Lipschitz & & & \checkmark & \checkmark & \checkmark & & & & CIFAR-10 & \\
             \rowcolor{tabgray}
            \t{RecurJac} \cite{zhang2019recurjac} & Lipschitz & & & \checkmark & \checkmark & \checkmark & & & & CIFAR-10 &  \\
            \t{CRC/CRT} \cite{singla2020second} & Curvature & & & & \checkmark & & & 3 & \checkmark & MNIST & \\
            \midrule
             \rowcolor{tabgray}
            \t{SDP Train}~\cite{raghunathan2018certified} & SDP & & & \checkmark & & & & & \checkmark & Synthetic & \\
            \t{SDP Verify}~\cite{raghunathan2018semidefinite} & SDP & & & \checkmark & & & & & & MNIST & Extend from \cite{raghunathan2018certified} \\ 
             \rowcolor{tabgray}
            \t{LMIVerify}~\cite{fazlyab2019safety} & SDP, dual & & & \checkmark & & & & & & CIFAR-10 & \\
            \t{PGD-SDP}~\cite{dvijotham2019efficient} & SDP, relax & & & \checkmark & & & & & & CIFAR-10 \\
            \midrule
             \rowcolor{tabgray}
            \t{DP} \cite{lecuyer2019certified} & DP, Rand. Smooth & &\checkmark & & \checkmark & \checkmark & & & \checkmark & ImageNet & \\
            \t{R\'enyi-divergence}~\cite{li2019certified} & Rand. Smooth & &\checkmark & & \checkmark & \checkmark & & & \checkmark & ImageNet & \\
             \rowcolor{tabgray}
            \t{Rand. Smooth} \cite{cohen2019certified} & Rand. Smooth & &\checkmark & & \checkmark & & & & \checkmark & ImageNet & \\
            \t{Unlabeled} \cite{carmon2019unlabeled} & Rand. Smooth & &\checkmark & & & & & & Only & ImageNet &  \\
             \rowcolor{tabgray}
            \t{Adversarial} \cite{salman2019provably} & Rand. Smooth & &\checkmark & & & & & & Only & ImageNet & \\
            \t{MACER} \cite{Zhai2020MACER:} & Rand. Smooth & &\checkmark & & & & & & Only & ImageNet &  \\
             \rowcolor{tabgray}
            \t{$\ell_0$-Lee} \cite{lee2019tight} & Rand. Smooth & &\checkmark & & & & \checkmark & & \checkmark & ImageNet & \\
            \t{$f$-divergence}~\cite{Dvijotham2020A} & Rand. Smooth & &\checkmark & \checkmark & \checkmark & \checkmark & \checkmark & & \checkmark & ImageNet &  \\
             \rowcolor{tabgray}
            \t{$\ell_1$-Teng}~\cite{teng2020ell} & Rand. Smooth & &\checkmark & & & \checkmark & & & \checkmark & ImageNet & \\
            \t{ADRE}~\cite{feng2020regularized} & Rand. Smooth & &\checkmark & & \checkmark & & & & \checkmark & ImageNet & \\
             \rowcolor{tabgray}
            \t{Zhang-Dual}~\cite{Zhang2020BlackBoxCW} & Rand. Smooth & &\checkmark & \checkmark & \checkmark & \checkmark & & & \checkmark & ImageNet & \\
            \t{All Shapes}~\cite{yang2020randomized} & Rand. Smooth & &\checkmark & \checkmark & \checkmark & \checkmark & & & \checkmark & ImageNet & \\
             \rowcolor{tabgray}
            \t{Low Rank enforcement}~\cite{awasthi2020adversarial} & Rand. Smooth & &\checkmark & \checkmark & \checkmark & & & 4 & \checkmark & CIFAR-10 &  \\
            \t{Consistency}~\cite{jeong2020consistency} & Rand. Smooth & &\checkmark & & & & & & Only & ImageNet &  \\
            \bottomrule
        \end{tabular}
        }
        
        {
            \flushleft \small
            \begin{minipage}{0.50\textwidth}
                \vspace{-0.6em}
                \tiny
                In ``Verification'' column,
                ``Complete'' means whether the verification approach is complete or not;
                ``Prob.'' means whether the approach is under probabilistic setting or not;
                each ``$\cL_p$'' column means whether the approach provides novel verification approach with experimental results under corresponding $\cL_p$ adversary.
                In ``Main Methodologies'' column: \\
                -~Branch: use branch-and-bound strategy.\\
                -~Relax: further relaxation on the ReLU linear bounds or SDP.\\
                -~Dual: derive from dual problem.\\
                -~DP: differential privacy.\\
                -~Rand. Smooth: probabilistic approach based on randomized models.\\
                -~Learned: the verification approach is learned from data statistics.
            \end{minipage}
            \hspace{0.03\textwidth}
            \begin{minipage}{0.45\textwidth}
                \tiny
                % \vspace{em}
                In ``Other'' column under ``Verification'': \\
                1.~Customized perturbation set, such as noise value differences in adjacent pixels to be $\le$ 0.05~(used in \cite{ehlers2017formal}); \\
                2.~Simple properties, such as limited number of changed neuron inputs in certain hidden layer used in \cite{10.1007/978-3-319-63387-9_1}.\\
                Scalability ranking: Synthetic $<$ MNIST $<$ CIFAR-10 $<$ ImageNet.\\
                Note that some approaches may be able to scale up to higher level, but not stated in their papers.\\
                3.~Only support smooth activation functions such as sigmoid, but not ReLU.\\
                4.~$\cL_\infty$ verification on projected low-dimensional space.\\
            \end{minipage}
        }
        
        \label{tab:approach-taxonogy}
    \end{table*}


% ================ Additional experiment results for arxiv version ================

% \ifnum\arxiv=1

\section{Full Experiment Details of Evaluation of Deterministic Verification Approaches}

    \label{sec:adx-full-exp-deterministic}

    In this appendix, we provide some more details about the evaluation of deterministic verification approaches~(\Cref{sec:exp-A}).

    \subsection{\textbf{Experimental Setup}}\hfill \\
        \para{Experiment Environment.} 
        For MNIST experiments, we run the evaluation on $24$-core Intel Xeon E5-2650 CPU running at \SI{2.20}{GHz} with single NVIDIA GeForce GTX 1080 Ti GPU.
        For CIFAR-10 experiments, we run the evaluation on $24$-core Intel Xeon Platinum 8259CL CPU running at \SI{2.50}{GHz} with single NVIDIA Tesla T4 GPU.
        The CIFAR-10 experiments use slightly faster running environment due to its larger scale.
        
        \para{Tool Implementation.}
        We implement our tool mainly in \texttt{PyTorch}~\cite{pytorch}.
        Some verification approaches use \texttt{keras}~\cite{keras} and \texttt{Tensorflow}~\cite{tensorflow}.
        For them, we implement a model translator from \texttt{PyTorch} directly to \texttt{keras} model, or to \texttt{onnx}~\cite{onnx} intermediate representation.
        The verification approaches reimplemented by ourselves use intrinsic \texttt{PyTorch} tensor computations, or \texttt{CVXPY}~\cite{cvxpy} + \texttt{Gurobi}~\cite{gurobi} solver when there is an optimization problem to solve.
        We test our implementation to ensure the correctness and high-efficiency.
        For verification approaches with hyperparameters, we use the hyperparameters used in their papers or their original implementations.
    
        % \para{Dataset.}
        % We evaluate these verification approaches on image classification datasets MNIST~\cite{lecuyer2019certified} and CIFAR-10~\cite{krizhevsky2009learning}.
            
        \para{Models.}
        We include $7$ different neural network structures from the literature and adapt them for each dataset.
        Among them, $3$~(\sc{FCNNa} - \sc{FCNNc}) are fully-connected neural networks, and $4$~(\sc{CNNa} - \sc{CNNd}) are convolutional neural networks.
        They are all feed-forward ReLU neural networks.
        The number of neurons ranges from $50$~(\sc{FCNNa}) to about $200,000$~(\sc{CNNd}).
        For each neural network structure, we train $5$ sets of weights: 
        \begin{itemize}
            \item \texttt{clean}~(on both MNIST and CIFAR-10): regular training; 
            \item \texttt{adv1}~(on MNIST)/\texttt{adv2}~(on CIFAR-10):\\ PGD adversarial training with $\epsilon = 0.1$ (on MNIST) or $\epsilon = 2/255$ (on CIFAR-10); 
            \item \texttt{adv3}~(on MNIST)/\texttt{adv8}~(on CIFAR-10):\\ PGD adversarial training with $\epsilon = 0.3$ (on MNIST) or $\epsilon = 8/255$ (on CIFAR-10);
            \item \texttt{cadv1}~(on MNIST)/\texttt{cadv2}~(on CIFAR-10):\\ \t{CROWN-IBP} training with $\epsilon = 0.1$ (on MNIST) or $\epsilon = 2/255$ (on CIFAR-10); 
            \item \texttt{cadv3}~(on MNIST)/\texttt{cadv8}~(on CIFAR-10):\\ \t{CROWN-IBP} training with $\epsilon = 0.3$ (on MNIST) or $\epsilon = 8/255$ (on CIFAR-10).
        \end{itemize}
            
        \input{tables/exp-A-models-stats}
        \input{tables/exp-A-models-originalacc}
            
        Here, $\epsilon$ is the $\cL_\infty$ radius of the adversarial examples.
        The PGD adversarial training~\cite{madry2017towards} is a strong empirical defense.
        We use $40$-step PGD in the PGD adversarial training.
        The \t{CROWN-IBP}~\cite{zhang2020towards} is a strong robust training approach.
        It achieves state-of-the-art certified robustness under $(\cL_\infty, 8/255)$ adversary.
        We choose these training configurations to reflect $3$ common types of models on which  verification approaches are used: normal models; empirical defense models; and robustly trained models.
        All models are trained to reach their expected accuracy or robustness.
        The model structures and statistics of number of neurons is shown in \Cref{table:expA-models-stats}.
        The model accuracy on original test set, and empirical robust accuracy under the PGD attack, is shown in \Cref{table:expA-models-originalacc}.
            
        \para{Evaluation protocol.}
        We present the performance of verification approaches by their \emph{robust accuracy} and \emph{average certified robustness radius} with respect to $\cL_\infty$ radius $\epsilon$.
            
        \vspace{1em}
        \emph{Robust Accuracy:}
        When measuring robust accuracy,
        the chosen radius $\epsilon$ for verification corresponds to the radius trained for defense.
        The robust accuracy is defined as $$\mathrm{robacc} := \dfrac{\text{\# samples verified to be robust}}{\text{\# number of all samples}}.$$
        On each dataset, we uniformly sample $100$ test set samples as the fixed set for evaluation.
        We further limit the running time to \SI{60}{s} per instance and count timeout instances as ``non-robust''.
        
        We also report the robust accuracy under empirical attack~(PGD attack), which gives an upper bound of robust accuracy, so we can estimate the gap between certified robust accuracy and accuracy of existing attack.
        % We remark that due to limited running time~(\SI{60}{s}) and different neural network models used in evaluation, the robust accuracy of some approaches differs much with the reported numbers, such as \t{k-ReLU}~\cite{singh2019beyond}, \t{RefineZono}~\cite{singh2018robustness}, \t{SDPVerify}~\cite{raghunathan2018semidefinite}, and \t{LMIVerify}~\cite{fazlyab2019safety}.
        
        \vspace{1em}
        \emph{Average Certified Robustness Radius:}
        We also evaluate the verification approaches by measuring their average certified robustness radius.
        The \emph{average certified robustness radius}~($\bar{r}$) stands for the average $\cL_\infty$ radius the verification approach can verify on the given subset of test set samples.
        We use the same uniformly sampled sets as in robust accuracy evaluation.
        To determine the best certified radius of each verification approach, we conduct a binary search process due to the monotonicity.
        Specifically, we do binary search on interval $[0,\,0.5]$ because the largest possible radius is $0.5$ for $[0,\,1]$ bounded input.
        If current radius $mid$ is verified to be robust, we update current best by $mid$ and let $l \gets mid$, if current radius $mid$ cannot be verified, we let $r \gets mid$, until we reach the precision $10^{-2}$ on MNIST or $10^{-3}$ on CIFAR-10, or time is up.
        For the evaluation of average certified robustness radius, since it involves multiple evaluations because of binary search, we limit the running time to \SI{120}{s} per input and record the highest certified radius it has been verified before the time is used up.
        The average certified robustness radius is evaluated on the same subset of test set samples as used for robust accuracy evaluation.
        
        We also report the smallest radius of adversarial samples found by empirical attack~(PGD attack), which gives an upper bound of certified robustness radius for us to estimate the gap.
        
        \vspace{1em}
        Throughout the evaluation, we use $100$-step PGD attack with step size equals to $\epsilon / 50$ where $\epsilon$ is the constrained $\cL_\infty$ attack radius.
            
    \subsection{\textbf{Full Results}}\hfill\\
        We present the full results as below.
        Besides robust accuracy and average certified robustness radius, we also report the running time per instance for each approach on both tasks respectively.
        Note that for robust accuracy evaluation, the verification is run once per instance with time limit \SI{60}{s}; 
        while for average certified robustness radius evaluation, the verification will be run multiple times due to the binary search, with overall time limit \SI{120}{s}.
        
        We summarize the references of corresponding result tables as below.
        
        \begin{table}[H]
            \centering
            \resizebox{0.8\linewidth}{!}{
            \begin{tabular}{cccc}
                \toprule
                Dataset & Evaluation Type & Results Table & Running Time Table \\
                \midrule
                \multirow{2}{*}{MNIST} & Robust Accuracy~($\mathrm{robacc}$) & \Cref{tab:exp-A-mnist-verify-robust-acc} & \Cref{tab:exp-A-mnist-verify-time} \\
                & Average certified robustness radius~($\bar r$) & \Cref{tab:exp-A-mnist-radius-robust-acc} & \Cref{tab:exp-A-mnist-radius-time} \\
                \hline
                \multirow{2}{*}{CIFAR-10} & Robust Accuracy~($\mathrm{robacc}$) & \Cref{tab:exp-A-cifar10-verify-robust-acc}\footnotemark & \Cref{tab:exp-A-cifar10-verify-time} \\
                & Average certified robustness radius~($\bar r$) & \Cref{tab:exp-A-cifar10-radius-robust-acc} & \Cref{tab:exp-A-cifar10-radius-time} \\
                \bottomrule
            \end{tabular}
            }
        \end{table}
        
        \footnotetext{Appeared in main text.}
    
        \input{tables/exp-A-mnist-verify-robust-acc}
        \input{tables/exp-A-mnist-verify-time}
        \input{tables/exp-A-mnist-radius-robust-acc}
        \input{tables/exp-A-mnist-radius-time}
        % \input{tables/exp-A-cifar10-verify-robust-acc}
        \input{tables/exp-A-cifar10-verify-time}
        \input{tables/exp-A-cifar10-radius-robust-acc}
        \input{tables/exp-A-cifar10-radius-time}
            
        \subsection*{Remarks.}
        Generally, the tendency on MNIST is the same as that on CIFAR-10.
        
        From these additional evaluations of average certified robustness radius, we can find that the average radius has better precision than robust accuracy.
        For example, on small models such as \sc{FNNa} and \sc{FNNb}, if measured by robust accuracy, the complete verification approaches and some linear relaxation-based approaches have almost the same precision~(see \cref{tab:exp-A-cifar10-verify-robust-acc}, the results of \t{Bounded MILP}, \t{AI$^2$}, \t{CROWN}, and \t{CNN-Cert}).
        However, if measured by average certified robustness radius, we can observe that complete verification approaches can certify much larger radius since they do not use any relaxations~(see \cref{tab:exp-A-cifar10-radius-robust-acc}, the result that \t{Bounded MILP} $\approx$ \t{AI$^2$} $>$ \t{CROWN} $\approx$ \t{CNN-Cert}).
        
        From the running time statistics, we further observe that a main cause of the failing cases~(i.e., $0$ robust accuracy or certified radius) for these approaches is the excessive verification time.
        In particular, since the evaluation of average certified robustness radius requires multiple times of verification for each instance, it suffers more severely from long verification time.

% \fi
